# Supplementary material for: Narrative Aligned Long Form Video Question Answering
Source: arXiv:2603.19481 source file (2026-03-19)
Supplement: Supplementary file 1 [file X_suppl.tex]

\clearpage
\setcounter{page}{1}
\maketitlesupplementary

\section{Dataset}

\subsection{Reasoning Dimension}
We generate Question–Answer–Evidence triplets capturing 7 reasoning types detailed below.
\paragraph{Causal Reasoning}
Causal reasoning refers to the ability to identify cause–effect relationships between events that are separated in time. A model must determine why an outcome occurred by grounding its explanation in earlier observable actions, conditions, or interactions that directly lead to the effect. 
\paragraph{Narrative Reasoning}
Narrative reasoning involves understanding how events unfold over time and how the story transitions from one state to another. The model must track progressions, shifts, and turning points, using a sequence of scenes that collectively show the evolution from an initial condition to a later one. 
\paragraph{Character-Centric Reasoning}
Character reasoning focuses on interpreting a character’s actions, decisions, and observable motivations.
The model must analyze behaviors, expressions, and repeated patterns to explain why a character acts a certain way. 
\paragraph{Thematic Reasoning}
Thematic reasoning captures a model’s ability to infer higher-level ideas or motifs that recur throughout the story.
The model must identify repeated visual patterns across multiple scenes and link them to a coherent theme.  
\paragraph{Goal-Based}
Goal-Based reasoning evaluates whether the model can understand a character’s goals, plans, and strategies.
It requires identifying a goal (explicit or implied) and the sequence of actions taken to pursue or achieve it. 
\paragraph{Social Reasoning}
Social reasoning reflects understanding of interpersonal relationships and how past interactions shape present reactions.
The model must ground answers in demonstrated dynamics such as trust, conflict, loyalty, or dominance—across multiple scenes. Valid evidence includes tone of interaction, supportive or hostile behavior, shared history, and reciprocal actions.
\paragraph{Hypothetical Reasoning}
Hypothetical reasoning involves evaluating alternative possibilities grounded in the constraints of the story world. The model must compare the actual outcome with a feasible alternative scenario, using what is visually established about objects, environment, and abilities. Valid evidence includes physical limitations, shown rules, or available options.

\subsection{Prompt}
To obtain the initial Question–Answer–Evidence triplets, we prompt the LLM with structured event descriptions from the movie, together with clear definitions of all reasoning types. We also supply exemplars for each category to anchor the model’s understanding and ensure consistent reasoning behavior. This setup helps the LLM frame questions that are grounded in observable events rather than external knowledge. The complete prompting template is provided below. The detailed prompts used for both the validator and refiner stages which are responsible for improving the quality of the dataset are also included.

\section{Experiment Section}
\label{sec:more_experiments}

\subsection{Metric}

\paragraph{LLM as a judge metric}
NA-VQA is evaluated along four dimensions: Comprehensiveness, Depth, Evidence Quality, and Reasoning. For the first three dimensions, we adopt the standardized evaluation metrics introduced in MovieCORE \cite{Faure2025MovieCORECR}, enabling consistent comparison with prior long-video benchmarks. For the Reasoning dimension, we design a dedicated LLM-based evaluation prompt that assesses whether the model demonstrates the intended causal, narrative, or character-centric reasoning. The full prompt is provided below.   

\begin{tcolorbox}[
    colback=white,
    colframe=blue!60!black,
    arc=10mm,
    boxrule=3pt,
    title={\small\bfseries Prompt for the Reasoning Metric},
    coltitle=white,
    colbacktitle=blue!60!black,
    fonttitle=\Large\bfseries
]

\tiny
\vspace{0.3cm}

You are an AI evaluator designed to assess the coherence and clarity of answers to video-based questions. Your task is to evaluate whether the predicted answer is well-structured and evaluate how well the predicted answer aligns with the ground truth in terms of reasoning quality.\\

INSTRUCTIONS: \\

Judge if the predicted answer’s explanation is logical, consistent, grounded, and free of hallucinations.\\

**Scoring** \\
Assign scores using the rubric below.\\
Reasoning Type Alignment – Does the answer reflect the correct reasoning type required by the question?\\

**0**: Completely misaligned reasoning approach.\\
**1**: Severely misaligned reasoning \\
**2**: Partially aligned reasoning with major gaps\\ 
**3**: Mostly aligned reasoning with some gaps \\
**4**: Well-aligned reasoning with minimal gaps.\\
**5**: Perfect reasoning alignment\\

%\textless Questions\textgreater

%\textless Options\textgreater

\end{tcolorbox}

%\begin{figure}[ht]
%    \includegraphics[width=\linewidth, height = 0.9\linewidth]{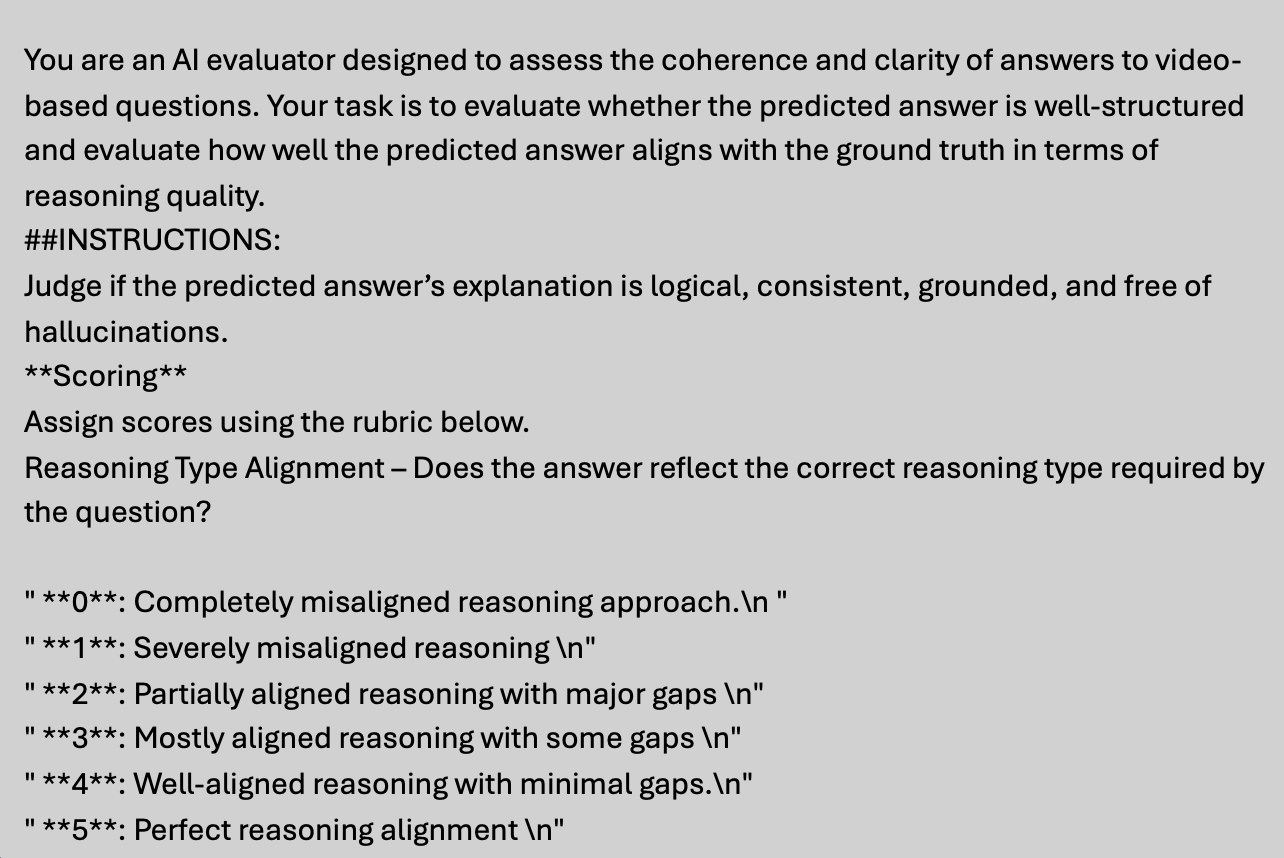}
%    \centering
%    \caption{Prompt for the Reasoning Metric.}
%    \label{fig:reasoningmetric}
%\end{figure}

\begin{table}[ht]
\centering
\caption{Performance comparison of different models on additional metrics. }
\label{tab:performance_previous}
\setlength{\tabcolsep}{2pt}
\tiny
\resizebox{0.45\textwidth}{!}{
\begin{tabular}{@{}l|cccc@{}}
\toprule
\textbf{Model} & \multicolumn{4}{c}{\textbf{Metrics}}\\
\cmidrule(l){2-5}
& BL-2 & MET & CID & BERT\\
\midrule
\rowcolor{gray!15}
\multicolumn{5}{c}{\textsc{\textbf{Proprietary Models}}} \\
\midrule
Claude Sonnet 4.5 & 0.0403 & 0.2372 & 0.0438 & 0.8435 \\
GPT-120B OSS & 0.0403 & 0.2372 & 0.0438 & 0.8435 \\
Qwen-243B & 0.0215 & 0.1707 & 0.0372 & 0.8345 \\
\midrule
\rowcolor{gray!15}
\multicolumn{5}{c}{\textsc{\textbf{Zero-Shot VLMs}}} \\
\midrule
LLaVA-OneVision (7B) & 0.0098 & 0.1048 & 0.0039 & 0.8559 \\
VideoLLaVA (7B) & 0.0228 & 0.1369 & 0.0220 & 0.8188 \\
Video-LLaMA3 (7B) & 0.0361 & 0.1721 & 0.0384 & 0.8498 \\
InternVL2 (7B) & 0.0345 & 0.1742 & 0.0310 & 0.8374 \\
InternVL2.5 (7B) & 0.0387 & 0.1927 & 0.0448 & 0.8350 \\
Qwen2.5-VL (7B) & 0.0343 & 0.1747 & 0.0327 & 0.8480 \\
\rowcolor{yellow!20}
\textbf{Video-NaRA} & 0.0354 & 0.1781 & 0.0398 & 0.8501\\
\midrule
\rowcolor{gray!15}
\multicolumn{5}{c}{\textsc{\textbf{Zero-Shot Long-Form VLMs}}} \\
\midrule
MovieChat (7B) & 0.0284 & 0.1527 & 0.0253 & 0.8388 \\
%MiniCPM-V 4.5 (7B) & 0.0237 & 0.1649 & 0.0294 & 0.8440 \\
VideoChat-Flash (7B) & 0.0167 & 0.1236 & 0.0032 & 0.8314 \\
\midrule
\rowcolor{gray!15}
\multicolumn{5}{c}{\textsc{\textbf{Fine-tuned Models}}} \\
\midrule
Qwen2.5-VL (FT) & 0.0338 & 0.1718 & 0.0244 & 0.8481 \\
\rowcolor{yellow!20}
\textbf{Video-NaRA} (FT) & 0.0366 & 0.1833 & 0.0458 & 0.8499\\
\bottomrule
\end{tabular}}
\end{table}
\subsection{Traditional Metrics}

In addition to using LLM-as-a-judge metrics to evaluate both reasoning quality and evidence grounding, we also report results on traditional metrics commonly used in prior work. Specifically, we include BLEU \cite{Papineni2002BleuAM}, CIDEr, METEOR \cite{Banerjee2005METEORAA}, and BERTScoreF1 \cite{Zhang2019BERTScoreET} scores. These metrics capture surface-level text similarity and measure how closely a model’s answer matches human-written references across n-gram overlap, sentence structure, and semantic alignment. While they do not fully reflect deeper narrative reasoning, they offer a standardized comparison point with existing long-video QA benchmarks. Across all of these metrics, our findings remain consistent \autoref{tab:performance_previous}. Video-NaRA (FT) outperformed Qwen2.5 VL (FT) across all evaluated metrics. Notably, Video-NaRA achieved the highest score on the CIDEr metric.

\subsection{Narrative Memory Construction}

Our model, Video-NaRA, takes both the clip descriptions and the raw frames to construct the narrative memory. Specifically, for each clip, we get the detail description that captures what is happening and who/what is involved. Description along with visual clip are passed to an MLLM that creates narrative slots based on shared entities, temporal continuity, and high-level scene semantics, allowing related events to be grouped even when they appear far apart in the movie. This gives us a compact yet expressive memory bank that reflects how the story unfolds and preserves the key evidence needed for retrieval. A detailed prompt for narrative-memory construction is below.
\vspace{30mm}

\begin{tcolorbox}[breakable,
    colback=white,
    colframe=blue!60!black,
    arc=10mm,
    boxrule=3pt,
    title={\small\bfseries Prompt for Narrative Memory Construction},
    coltitle=white,
    colbacktitle=blue!60!black,
    fonttitle=\Large\bfseries,
    fontupper=\small % or choose another size command
]

\tiny
You are an expert visual reasoning model organizing a movie into \{N\} fixed narrative slots.\\
Each slot represents one coherent storyline that unfolds across multiple clips.

\textbf{A narrative slot is defined by:}\\
\textbf{Character Continuity} -- the same people, animals, or key objects reappear visually.\\
\textbf{Goal or Action Continuity} -- the ongoing intention or action sequence remains consistent. (for example, a person running away, two people arguing, or a dog being rescued.)\\
\textbf{Plot/Sequence of Events} -- the logical cause and effect.

You are shown representative frames and description from each existing slot, followed by video from a new clip. Your task is to decide which slot the new clip most likely continues.

\textbf{Follow this reasoning process:}
\begin{itemize}
    \item Compare the new clip's visual content to each slot's frames.
    \item Look for shared characters, repeated actions, and similar emotional tone.
    \item Choose the slot that represents a continuation of the same story or situation.
    \item If no slot clearly matches (new characters, new goal, different emotion), assign it to the first unused slot (lowest ID without clips).
    \item Always output only one slot ID.
\end{itemize}

Return your decision \textbf{strictly in JSON format}, with no code fences, no extra text:

\{ "slot": \textless int \textgreater, "reason": "<brief explanation of your reasoning>" \}

Example valid outputs: \\
\{ "slot": 0, "reason": "Same woman and dog continue walking together" \} \\
\{ "slot": 3, "reason": "New character and setting, different tone" \}
\end{tcolorbox}

%\begin{figure}[ht]
%    \includegraphics[width=\linewidth]{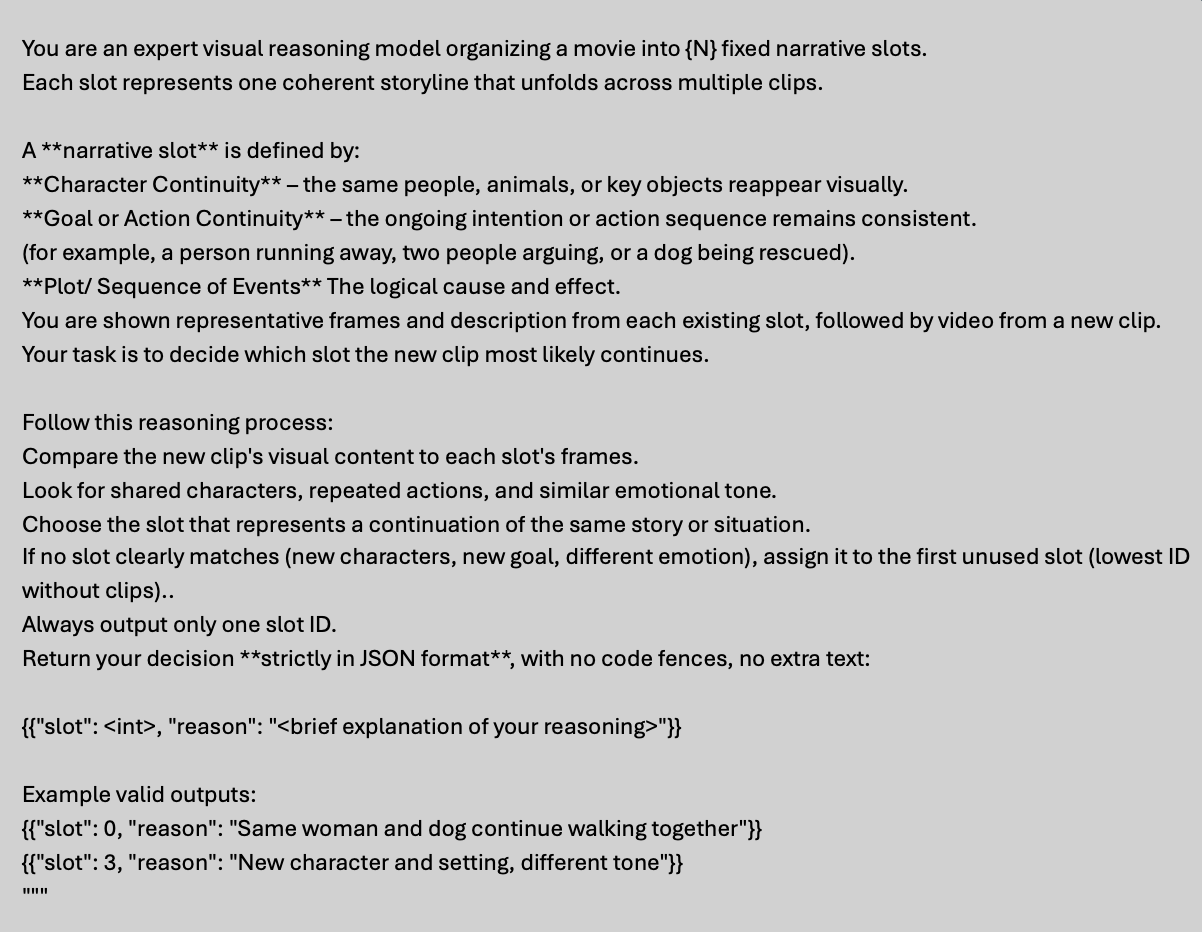}
%    \centering
%    \caption{Prompt for Narrative Memory Construction.}
%    \label{fig:narrative_memory}
%\end{figure}
%\vspace{-10mm}

\vspace{1 mm}
\begin{tcolorbox}[breakable,
    colback=white,
    colframe=blue!60!black,
    arc=10mm,
    boxrule=3pt,
    title={\small\bfseries Prompt for Refiner},
    coltitle=white,
    colbacktitle=blue!60!black,
    fonttitle=\Large\bfseries,
    fontupper=\small % Change to \normalsize or \footnotesize as needed
]
\tiny
You are an expert \textbf{Video QA Question–Answer–Evidence Refiner}. You will receive:
\begin{enumerate}
    \item A set of \textbf{movie events descriptions},
    \item An \textbf{original Question–Answer–Evidence triplet}, and
    \item \textbf{feedback} indicating scores of criteria and explanation.
\end{enumerate}

\textbf{Your task:}\\
Refine and correct the Question, Answer, and Evidence so they fully satisfy \textbf{all} criteria below while strictly adhering to the visual content described in the events.

\textbf{Grounding}
\begin{itemize}
    \item Only use information explicitly shown or visually inferable from the provided events.
    \item Do NOT add events, motivations, or facts not present in the events.
\end{itemize}

\textbf{Use Validation Feedback}
\begin{itemize}
    \item For each criterion marked with score 0, fix the issue in the refined QA-Evidence.
    \item If required evidence is missing in the events, adjust the question/answer accordingly. Do NOT invent new events.
\end{itemize}

\textbf{Quality Requirements}
\begin{itemize}
    \item \textbf{Video-Grounded}: The question must be answerable by watching the events alone.
    \item \textbf{Answer Faithfulness}: The answer must be strictly supported by the chosen evidence.
    \item \textbf{Events Completeness}: Include only the minimal events necessary; remove irrelevant ones.
    \item \textbf{Clarity \& Challenge}: The question must be clear, unambiguous, and non-trivial.
    \item \textbf{Reasoning Required}: The question must require narrative, causal, theme, reasoning, etc.
    \item \textbf{Character-Agnostic}: Do not use character names. Use visual descriptions only (e.g., ``the woman in the blue dress,'' ``the older man,'' etc.).
    \item \textbf{Content-Identifiability}: Everything must be visually interpretable without relying on dialogue unless described in the scenes.
\end{itemize}
Evidence must directly support the answer.
\end{tcolorbox}
\vspace{1 mm}
\begin{tcolorbox}[breakable,
    colback=white,
    colframe=blue!60!black,
    arc=10mm,
    boxrule=3pt,
    title={\small\bfseries Prompt for Validator},
    coltitle=white,
    colbacktitle=blue!60!black,
    fonttitle=\Large\bfseries,
    fontupper=\small % Change to \footnotesize or \normalsize if you prefer
]

\tiny
You are an expert video QA validation and correction assistant.\\
Your sole task is to critically evaluate a given Question, Answer, Evidence triplet based on a set of events from a movie.\\
You must follow these guidelines strictly:\\

\textbf{Evaluation Criteria:}\\
Please answer each question with 0, 1 and 2. Give a short, relevant explanation.

\begin{itemize}
    \item \textbf{Video-Grounded Framing}: Is the question framed so it can be answered by watching the video? (No external knowledge.)
    \item \textbf{Answer Faithfulness}: Is the answer factually correct \textbf{based only} on the provided events?
    \item \textbf{Events Completeness}: Are all the necessary events present to answer the question?
    \item \textbf{Minimal Events}: Are there any irrelevant events that do not add to the answer?
    \item \textbf{Clarity \& Challenge}: Is the question unambiguous and non-trivial (i.e., does it require interpretation, not surface detection)?
    \item \textbf{Reasoning Required}: Does the question require reasoning (narrative, causal, theme, etc.), not just recall?
    \item \textbf{Character-Agnostic}: Do the question, answer and evidences \textbf{avoid} using character names and instead describe observable content?
    \item \textbf{Content-Identifiability}: Can the question and answer be understood using \textbf{only the visual content} (not relying on dialogue)?
\end{itemize}
\end{tcolorbox}

%\begin{figure}[ht]
%    \includegraphics[width=\linewidth]{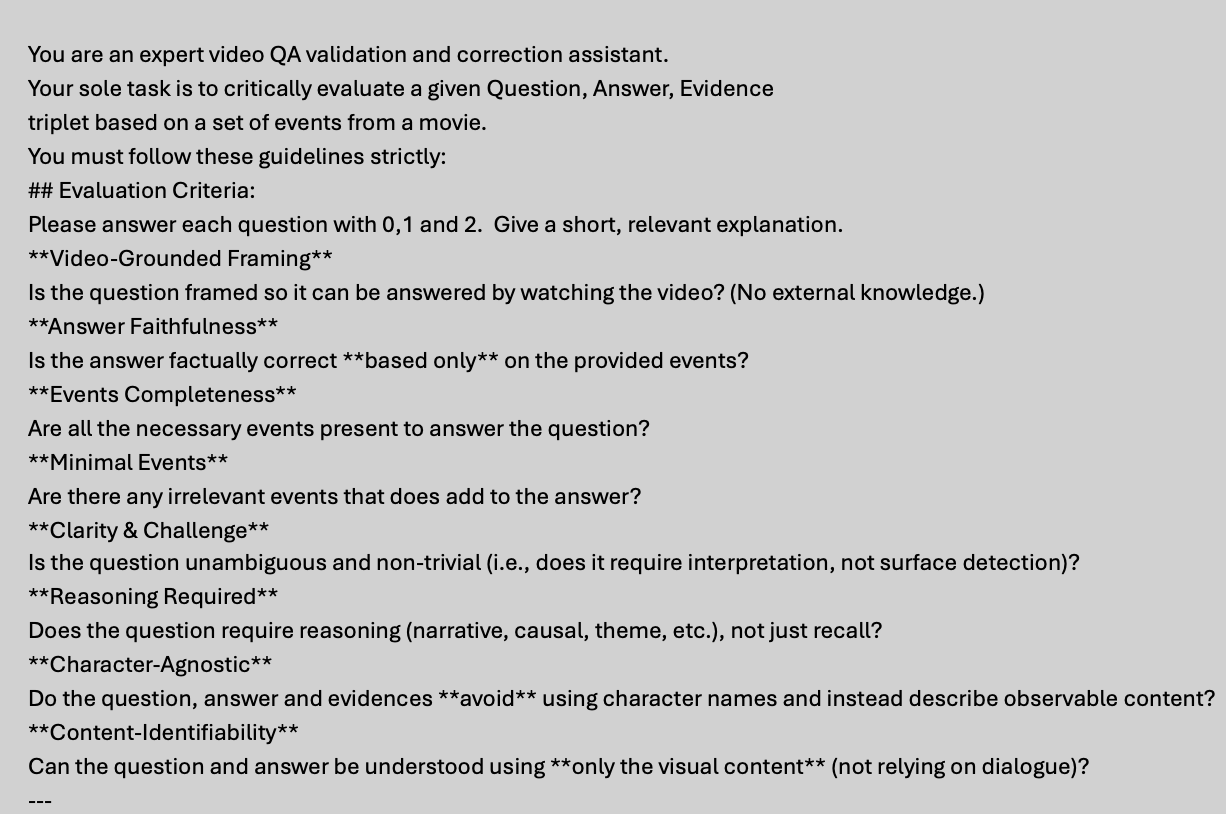}
%    \centering
%    \caption{Prompt for Validator.}
%    \label{fig:validator}
%\end{figure}

%\begin{figure}[ht]
%    \includegraphics[width=\linewidth]{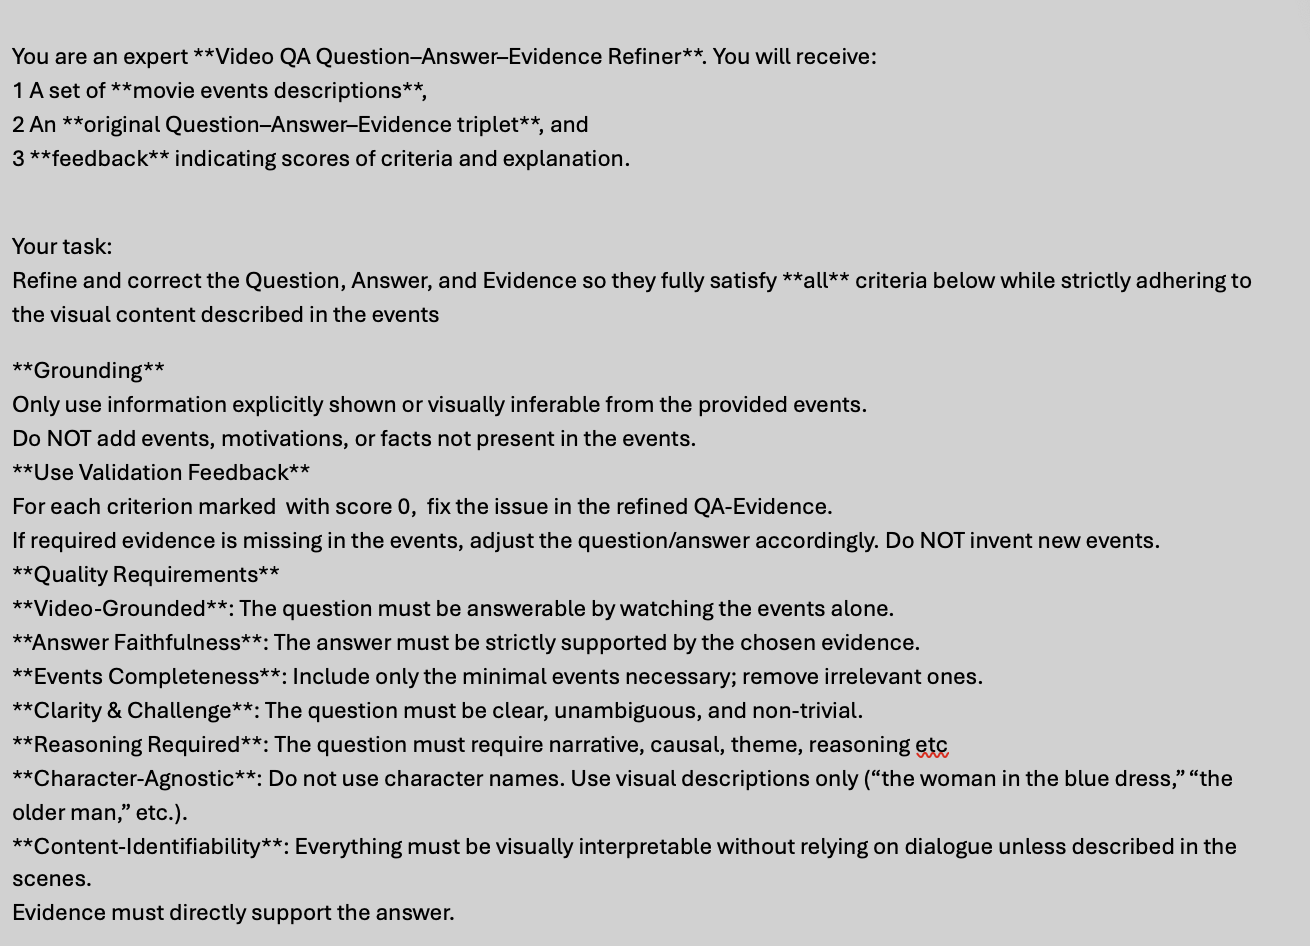}
%    \centering
%    \caption{Prompt for Refiner.}
%    \label{fig:refiner}
%\end{figure}

%\begin{figure*}
%    \includegraphics[width=0.7\linewidth, height = 1.2\linewidth]%{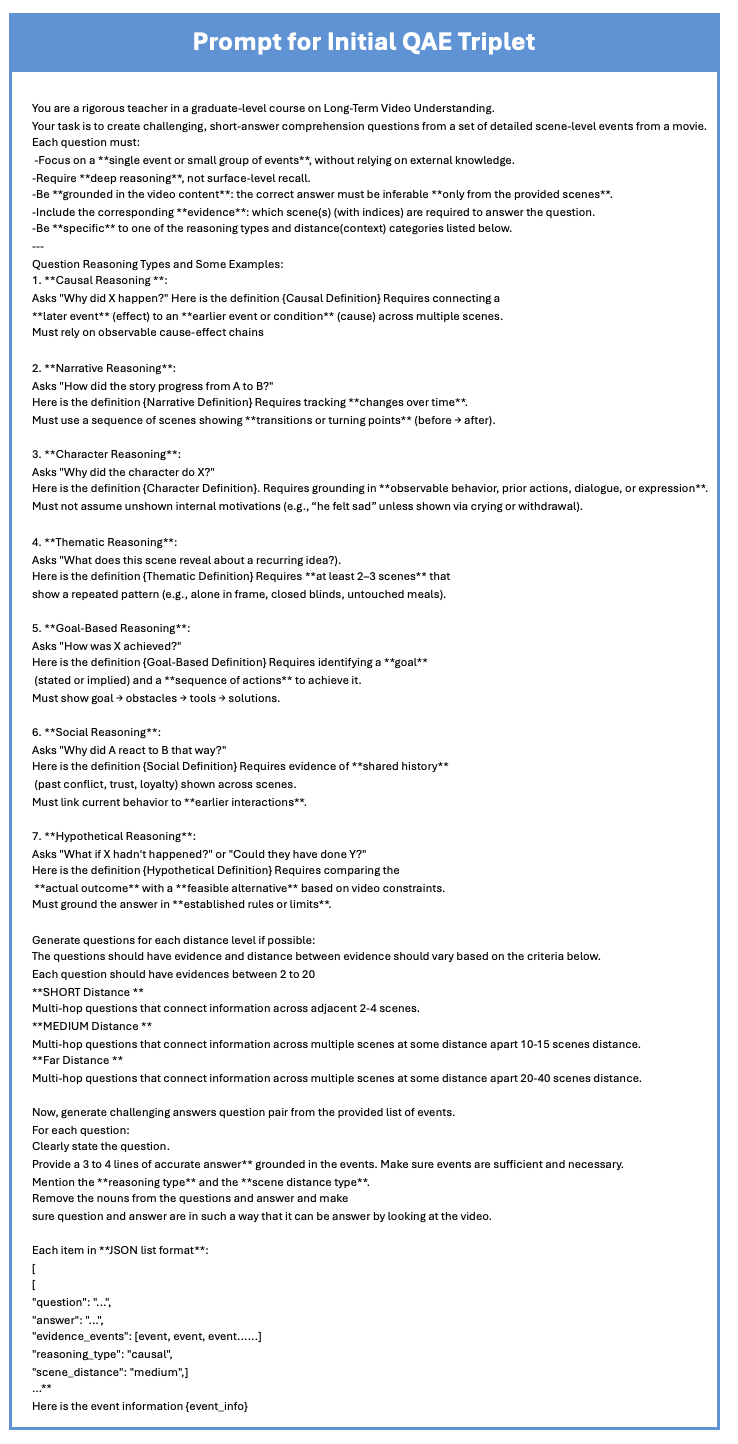}
%    \centering
%    \caption{Prompt for Initial QA.}
%    \label{fig:qa}
%\end{figure*}

\begin{figure*}[t]
\begin{tcolorbox}[
    enhanced,
    colback=white,
    colframe=blue!60!black,
    colbacktitle=blue!60!black,
    coltitle=white,
    fonttitle=\bfseries\small,
    title={Prompt for Initial Question Answer Evidence Triplet},
    arc=10mm,
    boxrule=3pt,
    left=10pt,
    right=10pt,
    top=5pt,
    bottom=10pt,
    toptitle=8pt,
    bottomtitle=8pt,
    width=0.9\textwidth
]

\tiny
\textbf{You are a rigorous teacher in a graduate-level course on Long-Term Video Understanding.}

Your task is to create challenging, short-answer comprehension questions from a set of detailed scene-level events from a movie.\\

Each question must:
\begin{itemize}
    \item Focus on a \textbf{single event or small group of events}, without relying on external knowledge.
    \item Require \textbf{deep reasoning}, not surface-level recall.
    \item Be \textbf{grounded in the video content}: the correct answer must be inferable \textbf{only from the provided scenes}.
    \item Include the corresponding \textbf{evidence}: which scene(s) (with indices) are required to answer the question.
    \item Be \textbf{specific} to one of the reasoning types and distance(context) categories listed below.
\end{itemize}

\hrulefill

\textbf{Question Reasoning Types and Some Examples:}

\begin{enumerate}
    \item \textbf{Causal Reasoning}: 
    Asks "Why did X happen?" Here is the definition \{Causal Definition\} Requires connecting a 
    later event (effect) to an earlier event or condition (cause) across multiple scenes. 
    Must rely on observable cause-effect chains.\\
    
    \item \textbf{Narrative Reasoning}: 
    Asks "How did the story progress from A to B?" 
    Here is the definition \{Narrative Definition\} Requires tracking changes over time. 
    Must use a sequence of scenes showing transitions or turning points (before → after).\\
    
    \item \textbf{Character Reasoning}: 
    Asks "Why did the character do X?" 
    Here is the definition \{Character Definition\}. Requires grounding in observable behavior, prior actions, dialogue, or expression. 
    Must not assume unshown internal motivations (e.g., "he felt sad" unless shown via crying or withdrawal).\\
    
    \item \textbf{Thematic Reasoning}: 
    Asks "What does this scene reveal about a recurring idea?" 
    Here is the definition \{Thematic Definition\} Requires at least 2–3 scenes that 
    show a repeated pattern (e.g., alone in frame, closed blinds, untouched meals).\\
    
    \item \textbf{Goal-Based Reasoning}: 
    Asks "How was X achieved?" 
    Here is the definition \{Goal-Based Definition\} Requires identifying a goal
    (stated or implied) and a sequence of actions to achieve it. 
    Must show goal → obstacles → tools → solutions.\\
    
    \item \textbf{Social Reasoning}: 
    Asks "Why did A react to B that way?" 
    Here is the definition \{Social Definition\} Requires evidence of shared history
    (past conflict, trust, loyalty) shown across scenes. 
    Must link current behavior to \textbf{earlier interactions}.\\
    
    \item \textbf{Hypothetical Reasoning}: 
    Asks "What if X hadn't happened?" or "Could they have done Y?" 
    Here is the definition \{Hypothetical Definition\} Requires comparing the
    actual outcome with a feasible alternative based on video constraints. 
    Must ground the answer in established rules or limits.\\
\end{enumerate}

\hrulefill

\textbf{Generate questions for each distance level if possible:}\\

The questions should have evidence and distance between evidence should vary based on the criteria below. 
Each question should have evidences between 2 to 20.\\

\textbf{SHORT Distance:} Multi-hop questions that connect information across adjacent 2-4 scenes.\\

\textbf{MEDIUM Distance:} Multi-hop questions that connect information across multiple scenes at some distance apart 10-15 scenes distance.\\

\textbf{FAR Distance:} Multi-hop questions that connect information across multiple scenes at some distance apart 20-40 scenes distance.\\

\hrulefill

\textbf{Now, generate challenging answers question pair from the provided list of events.} \\

For each question:
\begin{itemize}
    \item Clearly state the question.\\
    \item Provide a 3 to 4 lines of \textbf{accurate answer} grounded in the events. Make sure events are sufficient and necessary.\\
    \item Mention the \textbf{reasoning type} and the \textbf{scene distance type}.\\
    \item Remove the nouns from the questions and answer and make sure question and answer are in such a way that it can be answered by looking at the video.\\
\end{itemize}

\textbf{Each item in JSON list format:}
\begin{verbatim}
[
  {
    "question": "...",
    "answer": "...",
    "evidence_events": [event, event, event......],
    "reasoning_type": "causal",
    "scene_distance": "medium"
  },
  ...
]
\end{verbatim}

Here is the event information \{event\_info\}

\end{tcolorbox}
\end{figure*}

\begin{figure*}[ht!]
    \centering
    \includegraphics[width=0.8\linewidth]{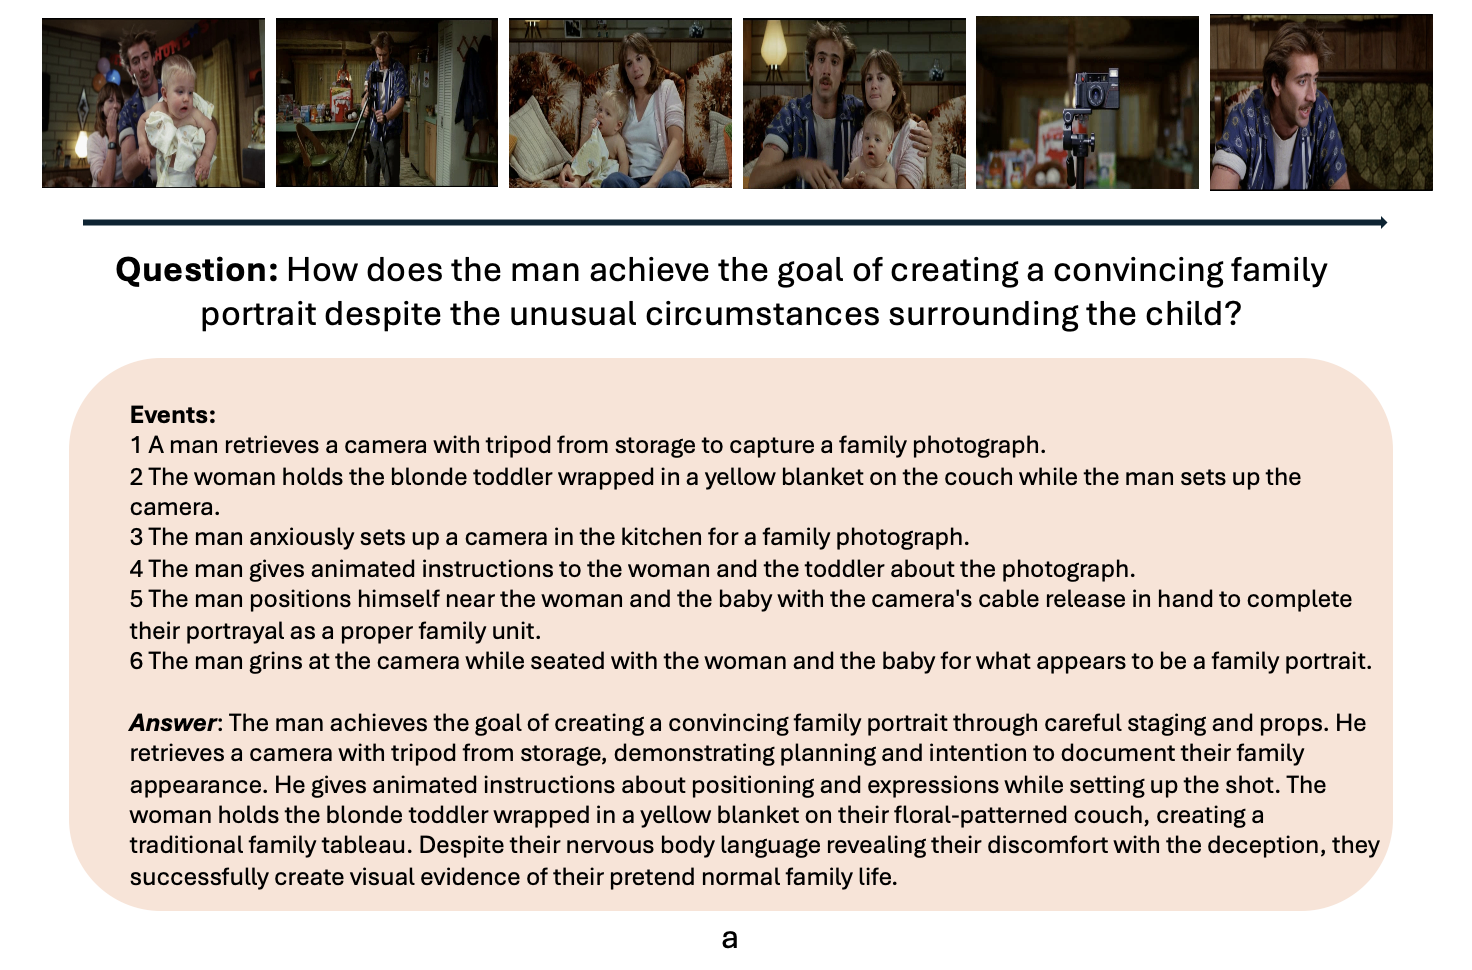}
    \label{fig:sample1}

    \vspace{1em} % space between images

    \includegraphics[width=0.8\linewidth]{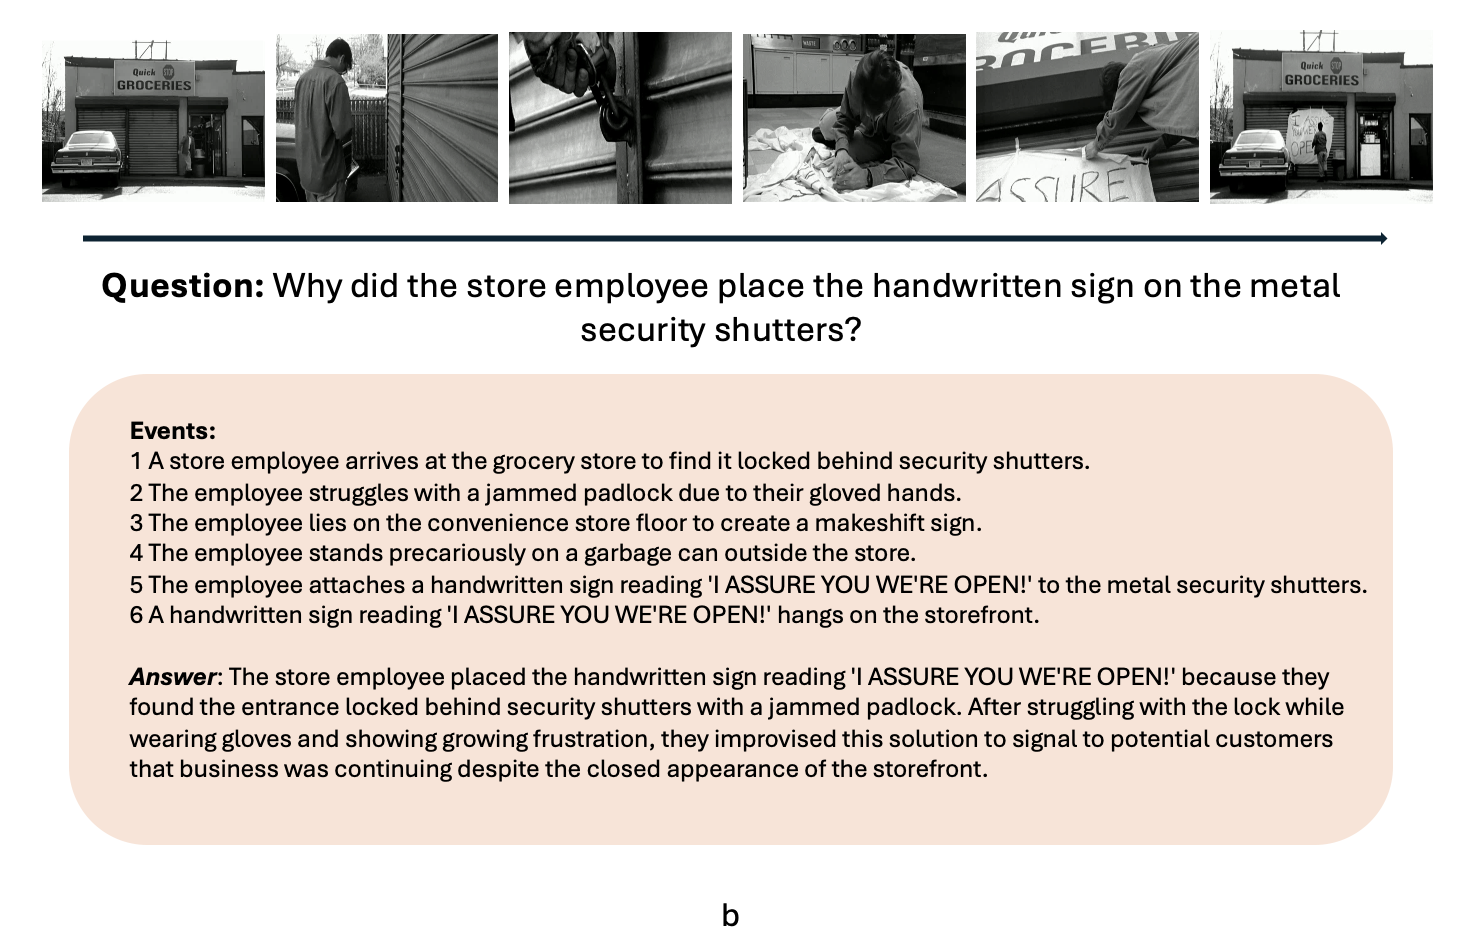}
    \caption{Additional samples from our NA-VQA dataset.}
    \label{fig:sample2}
\end{figure*}
